# Supplementary material for: Interpretable Trade-offs Between Robot Task Accuracy and Compute Efficiency
Source: arXiv:2108.01235 source file (2021-08-03)
Supplement: Supplementary file 1 [file appendix.tex]

\subsection{DNN Architecture}
\label{appsubsec:DNN_arch}
In this section, we describe the architectures of the DNNs used to evaluate our model selection policy, as described in Subsection \ref{subsec:app_dnn}. The ResNet-18 DNN architecture that works on full-sized images is as follows: A trained ResNet-18 feature extractor, with an additional linear layer that has two output features. The small DNN architecture that works on downsampled images is as follows: two 1-D convolutional layer with a 1-D MaxPool layer in the middle, finally sent through linear layer with sigmoid activation function.
